# Supplementary material for: Viscometric Functions and Rheo-optical Properties of Dilute Polymer Solutions: Comparison of FENE-Fraenkel Dumbbells with Rodlike Models
Source: arXiv:2007.00184 ancillary file (2020-09-08)
Supplement: Supplementary file 1 [file JNNFM-S-20-00216R1_SI.pdf]

**Supporting Information for:**

# Viscometric Functions and Rheo-optical Properties of a Dilute Solution: Comparison of FENE-Fraenkel Dumbbells with Rodlike Models

I. Pincus,[1] A. Rodger,[2] and J. Ravi Prakash[1, a)]

[1)] *Department of Chemical Engineering, Monash University, Melbourne, VIC 3800, Australia*

[2)] *Macquarie University Department of Molecular Sciences, Sydney, Australia*

[a)] Electronic mail: ravi.jagadeeshan@monash.edu

## I. Dumbbell Models

### A. Diffusion equation for springs

We begin with the equation of continuity for the bead-bead connector vector distribution function $\psi(\boldsymbol{Q}, t)$, given as:[1]

$$\frac{\partial \psi}{\partial t} = -\left( \frac{\partial}{\partial \boldsymbol{Q}} \cdot [\![\dot{\boldsymbol{Q}}]\!] \psi \right) \tag{1}$$

which says that the rate of change of $\psi$ at a particular $\boldsymbol{Q}$ is equal to the spatial derivative of $\psi$ times the velocity-averaged connector vector velocity $[\![\dot{\boldsymbol{Q}}]\!]$. For the spring, we can find $[\![\dot{\boldsymbol{Q}}]\!]$ by considering a force balance over each bead. The overall force on each bead at a given moment is the sum of three general forces, the hydrodynamic force $\boldsymbol{F}^{(h)}$, the Brownian or random force $\boldsymbol{F}^{(b)}$ and the connector vector spring force $\boldsymbol{F}^{(c)}$. By assuming a Maxwellian velocity distribution for the Brownian force and including hydrodynamic interactions, it can be shown that:[1]

$$[\![\dot{\boldsymbol{Q}}]\!] = [\boldsymbol{\kappa} \cdot \boldsymbol{Q}] + \left[ (\boldsymbol{\delta} - \zeta \boldsymbol{\Omega}) \cdot \left( -\frac{2kT}{\zeta} \frac{\partial}{\partial \boldsymbol{Q}} \ln \psi - \frac{2}{\zeta} \boldsymbol{F}^{(c)} \right) \right] \tag{2}$$

where $\zeta = 6\pi\eta_s a$ (Stokes drag) and $\boldsymbol{\Omega}$ is the tensor describing hydrodynamic interactions between the beads. The beads then have hydrodynamic radius $a$ and the solvent has Newtonian viscosity $\eta_s$. $\boldsymbol{\Omega}$ has the general form

$$\boldsymbol{\Omega}(\boldsymbol{Q}) = \frac{3a}{4\zeta Q} \left( A\boldsymbol{\delta} + B \frac{\boldsymbol{QQ}}{Q^2} \right) \tag{3}$$

where the constants $A$ and $B$ must be chosen carefully to ensure the tensor correctly describes the bead-bead interaction while also remaining positive-semidefinite.[2] A common choice is the Rotne-Prager-Yamakawa (RPY) tensor, which has two separate branches depending on whether the bead separation is greater or less than $2a$:

$$A = 1 + \frac{2}{3}\left(\frac{a}{Q}\right)^2, B = 1 - 2\left(\frac{a}{Q}\right)^2 \text{ for } Q \geq 2a \tag{4a}$$

$$A = \frac{4}{3}\left(\frac{Q}{a}\right) - \frac{3}{8}\left(\frac{Q}{a}\right)^2, B = \frac{1}{8}\left(\frac{Q}{a}\right)^2 \text{ for } Q < 2a \tag{4b}$$

We have used the RPY form throughout this study for both spring-dumbbells and rod-dumbbells. Another form suggested by Öttinger[2] for the specific case of dumbbells is the regularised Oseen-Burgers (ROB) tensor, and we have verified that our results are indistinguishable to within simulation error between the ROB and RPY tensors.

Upon substitution of Eq. (2) into Eq. (1), we arrive at the diffusion equation for the configurational distribution function:

$$\frac{\partial \psi}{\partial t} = -\frac{\partial}{\partial \boldsymbol{Q}} \cdot [\boldsymbol{\kappa} \cdot \boldsymbol{Q}]\psi + \frac{\partial}{\partial \boldsymbol{Q}} \cdot \left[(\boldsymbol{\delta} - \zeta\boldsymbol{\Omega}) \cdot \frac{2kT}{\zeta}\frac{\partial}{\partial \boldsymbol{Q}} \ln \psi\right]\psi + \frac{\partial}{\partial \boldsymbol{Q}} \cdot \left[(\boldsymbol{\delta} - \zeta\boldsymbol{\Omega}) \cdot \frac{2}{\zeta}\boldsymbol{F}^{(c)}\right]\psi \tag{5}$$

The aim is then to get the equation above into the general form of the Fokker-Planck equation, as it can then be interpreted as a stochastic differential equation using Îto's method. To do so we apply the identity:[3]

$$\frac{\partial}{\partial \boldsymbol{Q}} \cdot \left[\boldsymbol{L} \cdot \frac{\partial f}{\partial \boldsymbol{Q}}\right] = \frac{\partial}{\partial \boldsymbol{Q}}\frac{\partial}{\partial \boldsymbol{Q}} : [\boldsymbol{L}^T f] - \frac{\partial}{\partial \boldsymbol{Q}} \cdot \left[f\frac{\partial}{\partial \boldsymbol{Q}} \cdot \boldsymbol{L}^T\right] \tag{6}$$

where $\boldsymbol{L}$ is a rank-2 tensor and $f$ is some scalar function. Then, by noting that $(\boldsymbol{\delta} - \zeta\boldsymbol{\Omega})$ is symmetric, and further that $\boldsymbol{\nabla} \cdot \boldsymbol{\Omega} = 0$ for the Oseen-Burgers tensor[2] (which is also the case for the ROB and RPY tensors):

$$\frac{\partial \psi}{\partial t} = -\frac{\partial}{\partial \boldsymbol{Q}} \cdot \left\{\boldsymbol{\kappa} \cdot \boldsymbol{Q} - (\boldsymbol{\delta} - \zeta\boldsymbol{\Omega}) \cdot \frac{2}{\zeta}\boldsymbol{F}^{(c)}\right\}\psi + \frac{2k_{\mathrm{B}}T}{\zeta}\frac{\partial}{\partial \boldsymbol{Q}}\frac{\partial}{\partial \boldsymbol{Q}} : [\boldsymbol{\delta} - \zeta\boldsymbol{\Omega}]\psi \tag{7}$$

This Fokker-Planck equation forms the basis of the Brownian Dynamics simulations, which are used to solve for $\psi$.

### B. Diffusion Equation for Rods

Note that for a rod, the connector vector has a fixed length, and so can be written as $\boldsymbol{Q} = L\boldsymbol{u}$, where $\boldsymbol{u}$ is the radial unit vector in spherical coordinates. The continuity

equation then reduces to the form

$$\frac{\partial \psi}{\partial t} = -\left( \frac{\partial}{\partial \boldsymbol{u}} \cdot [\![\dot{\boldsymbol{u}}]\!] \psi \right) \tag{8}$$

when $\psi = \psi(\boldsymbol{u}(t), t)$.

The expression for $[\![\dot{\boldsymbol{u}}]\!]$ for the rod is similar to that for the spring, except that there is no spring force $\boldsymbol{F}^{(c)}$, and the forces must be projected onto the $\phi$ and $\theta$ components through multiplication by $(\boldsymbol{\delta} - \boldsymbol{uu})$ (where $\boldsymbol{\delta}$ is the unit rank-2 tensor). It can be shown[1] that this force projection gives the following expression for the velocity-averaged radial unit vector velocity, when the hydrodynamic interaction is mediated via the RPY tensor as per Eq. (4):

$$[\![\dot{\boldsymbol{u}}]\!] = [\boldsymbol{\kappa} \cdot \boldsymbol{u}] - [\boldsymbol{\kappa} : \boldsymbol{uuu}] - \frac{2kT(1 - Ah)}{\zeta L^2} \frac{\partial}{\partial \boldsymbol{u}} \ln \psi \tag{9}$$

where $h_R^* = 3a/4L$ is the hydrodynamic interaction parameter for a bead-rod dumbbell and $A$ is the same as that given in Eq. (4) with $Q = L$. This expression can then be substituted in to the continuity equation (8), giving

$$\frac{\partial}{\partial t} \psi = \frac{2}{\lambda_2^{(1)}} \left( \frac{\partial}{\partial \boldsymbol{u}} \cdot \frac{\partial}{\partial \boldsymbol{u}} \psi \right) - \left( \frac{\partial}{\partial \boldsymbol{u}} \cdot [\boldsymbol{\kappa} \cdot \boldsymbol{u} - \boldsymbol{\kappa} : \boldsymbol{uuu}] \psi \right) \tag{10}$$

in which we have used the time constant $\lambda_2^{(1)} = (\zeta L^2/kT)[1 - h_R^*(1 + 2a^2/3L^2)]^{-1}$ for bead-rod dumbbells with RPY HI. Here we use $\lambda_2^{(1)}$ to refer to the diffusion equation time constant for a dumbbell (with two beads). Note that we actually obtain the same general form of the diffusion equation for any rigid system with only two degrees of (orientational) freedom, such as a multibead-rod, prolate spheroid, cylinder or slender-body. These models differ only in the form of $\lambda$, which varies with the rotational friction. Furthermore, there are two time constants which characterise these systems, $\lambda^{(1)}$, which appears in diffusion equations similar to Eq. (10), and $\lambda^{(2)}$, which determines how the stress tensor varies with the distribution function in flow (as can be seen in Eq. 23 in section II A below). For a multibead-rod model, we can further denote $\lambda_N^{(1)}$ and $\lambda_N^{(2)}$ as the time constants for an $N$-bead rigid rod.

## II. Simulation Methodology

Here we use a semi-implicit predictor-corrector scheme based on solving a cubic polynomial, as suggested by Öttinger[2] and then applied to multi-bead chains with HI by Hsieh et al.[4] as well as Prabhakar and Prakash,[5] who also included excluded-volume interactions. Here we assume that all quantities are in the Hookean non-dimensional form, and so drop the * and $_{\mathrm{H}}$ superscripts and subscripts. Additionally, we will define $\alpha = \delta Q_{\mathrm{H}}^{*2}$, such that $\alpha$ is equivalent to the FENE-spring $b$-parameter (see,[1] section 13.5).

We begin with the Fokker-Planck Eq. (7) non-dimensionalised via Hookean units. In Îto's interpretation, there is an equivalence between the above Fokker-Planck equation and the following stochastic differential equation:[2]

$$d\boldsymbol{Q} = \left(\boldsymbol{\kappa} \cdot \boldsymbol{Q} - [\boldsymbol{B}(\boldsymbol{Q}) \cdot (\boldsymbol{B}(\boldsymbol{Q}))^T] \cdot \frac{1}{2}\boldsymbol{F}^{(c)}\right) dt + \boldsymbol{B}(\boldsymbol{Q}) d\boldsymbol{W} \tag{11}$$

where $d\boldsymbol{W}$ is a Wiener process and $\boldsymbol{B}(\boldsymbol{Q}) \cdot (\boldsymbol{B}(\boldsymbol{Q}))^T = \boldsymbol{\delta} - \zeta\boldsymbol{\Omega}$. In this case we can choose $\boldsymbol{B}(\boldsymbol{Q})$ to have the form:[2]

$$\boldsymbol{B}(\boldsymbol{Q}) = \boldsymbol{\delta}\sqrt{1 - \frac{3a}{4Q}A} + \frac{\boldsymbol{Q}\boldsymbol{Q}}{(Q)^2}\left(\sqrt{1 - \frac{3a}{4Q}(A+B)} - \sqrt{1 - \frac{3a}{4Q}A}\right) \tag{12}$$

Note that $A$ and $B$ (defined in Eq. (4)) are already dimensionless, so converting them to $A_{\mathrm{H}}^*$ and $B_{\mathrm{H}}^*$ is simply a matter of substituting $a \to a_{\mathrm{H}}^*$ and $Q \to Q_{\mathrm{H}}^*$.

We can now describe our numerical integration method for the above stochastic differential equation. This is broken into 3 main parts, the first of which is a predictor step based on the value of variables at the beginning of the timestep. We adopt the convention that any quantity with a bar (e.g. $\bar{\boldsymbol{Q}}$) represents a predicted quantity, while the subscripts $j$ and $j+1$ refer to the beginning and the end of the timestep. We can then write Eq. (11) in the following approximate finite difference form:

$$\begin{aligned}\bar{\boldsymbol{Q}}_{j+1} &= \boldsymbol{Q}_j + \left(\boldsymbol{\kappa} \cdot \boldsymbol{Q}_j - \frac{1}{2}[\boldsymbol{B}(\boldsymbol{Q}_j) \cdot (\boldsymbol{B}(\boldsymbol{Q}_j))^T] \cdot \boldsymbol{F}_j^{(c)}\right) \Delta t + \boldsymbol{B}(\boldsymbol{Q}_j) \cdot \Delta \boldsymbol{W}_j \\ &\equiv \boldsymbol{Q}_j + \left(\boldsymbol{\kappa} \cdot \boldsymbol{Q}_j - \frac{1}{2}[\boldsymbol{\delta} - \zeta\boldsymbol{\Omega}] \cdot \boldsymbol{F}_j^{(c)}\right) \Delta t + \boldsymbol{B}(\boldsymbol{Q}_j) \cdot \Delta \boldsymbol{W}_j\end{aligned} \tag{13}$$

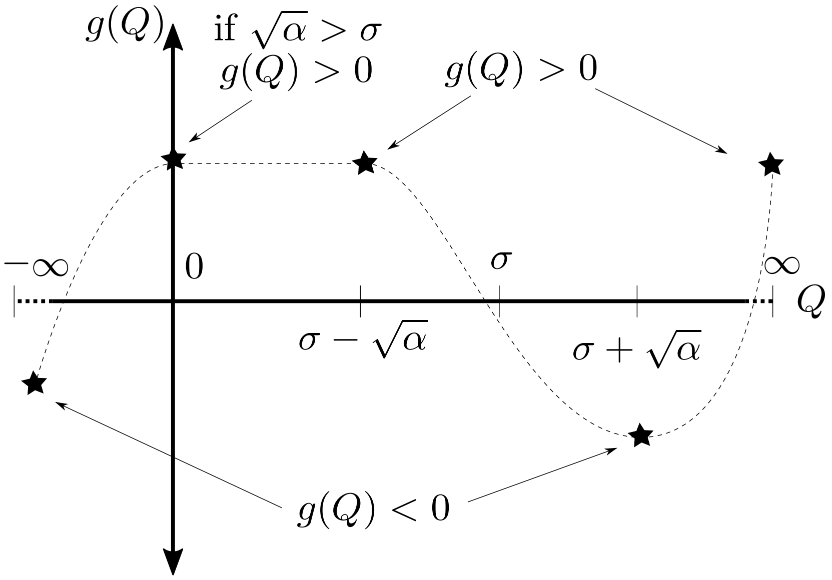


FIG. S1. Visualisation of the range of the cubic equation, showing why there must be a real root between $\sigma - \sqrt{\alpha}$ and $\sigma + \sqrt{\alpha}$. The key insight is that $g(Q)$ must be negative at $\sigma + \sqrt{\alpha}$ and must be positive at the larger of $\sigma - \sqrt{\alpha}$ and 0, with no inflection points within this range. Therefore, we know that one root must lie in that range.

We then apply a corrector step using the previous predictor value, treating the force law implicitly. We don't recalculate the HI tensor, since the change is negligible over the course of a timestep and doing so was found to have no effect upon accuracy. The predictor step can be expressed as follows:

$$\boldsymbol{Q}_{j+1} + \frac{\Delta t}{4}\boldsymbol{F}^{(c)}_{j+1} = \boldsymbol{Q}_j + \frac{1}{2}\bigg(\boldsymbol{\kappa} \cdot (\boldsymbol{Q}_j + \bar{\boldsymbol{Q}}_{j+1}) - [\boldsymbol{B}(\boldsymbol{Q}_j) \cdot (\boldsymbol{B}(\boldsymbol{Q}_j))^T] \cdot \boldsymbol{F}^{(c)}_j + \frac{1}{2}\boldsymbol{F}^{(c)}_j\bigg)\Delta t + \boldsymbol{B}(\boldsymbol{Q}_j) \cdot \Delta \boldsymbol{W}_j \quad (14)$$

where all terms depending on the final spring force have been moved to the LHS. This makes the implicit assumption that the spring force is approximately equal at the beginning and end of the timestep, such that $-[\boldsymbol{B} \cdot \boldsymbol{B}^T] \cdot \boldsymbol{F}^{(c)}_j + \boldsymbol{F}^{(c)}_{j+1} \approx -[\boldsymbol{\delta} - \zeta\boldsymbol{\Omega}] \cdot \boldsymbol{F}^{(c)}_j + \boldsymbol{F}^{(c)}_j = \zeta\boldsymbol{\Omega} \cdot \boldsymbol{F}^{(c)}_j$. If we then denote the RHS of Eq. (14) by $\boldsymbol{Y}$ and give the full form of $\boldsymbol{F}^{(c)}_{j+1}$, then:

$$\boldsymbol{Q}_{j+1} + \frac{\Delta t}{4}\left[\frac{Q_{j+1} - \sigma}{1 - (Q_{j+1} - \sigma)^2/\alpha}\frac{\boldsymbol{Q}_{j+1}}{Q_{j+1}}\right] = \boldsymbol{Y} \quad (15)$$

If we denote $\hat{\boldsymbol{u}}$ as a unit vector in the $\boldsymbol{Y}$ direction, then we can take the magnitude of

both sides and solve implicitly for $Q_{j+1}$ using the following cubic equation:

$$0 = Q^3 - Q^2[2\sigma + Y] - Q[\alpha - \sigma^2 - 2Y\sigma + \beta] + [\beta\sigma + Y\alpha - Y\sigma^2] = g(Q) \qquad (16)$$

where $\beta = 0.25\alpha\Delta t$ and $Q \equiv Q_{j+1}$. If we give Eq. (16) the label $g(Q) = 0$, then we can evaluate $g(Q)$ at different points to determine the ranges for the roots:

- $g(\infty) > 0$
- $g(\sigma + \sqrt{\alpha}) = -\beta\sqrt{\alpha} < 0$
- $g(\sigma - \sqrt{\alpha}) = \beta\sqrt{\alpha} > 0$
- $g(0) = \beta + (\alpha - \sigma^2) \cdot Y$, so if $\sqrt{\alpha} \geq \sigma$, then $g(0) > 0$
- $g(-\infty) < 0$

Therefore, one of the roots of the equation is always positive with an upper bound of $\sigma + \sqrt{\alpha}$ and a lower bound of the larger of 0 or $\sigma - \sqrt{\alpha}$, which is chosen as the value of $Q$. This is displayed graphically in Fig. S1. The other two roots will be outside of this range, but also real. Note that this implies that when $\sigma = 0$, we recover the behaviour of a FENE spring, where we can say $\alpha \equiv b$, and clearly $\sqrt{b} > \sigma = 0$.

Finally, we set $\boldsymbol{Q} = Q\hat{\boldsymbol{u}} \equiv Q\boldsymbol{Y}/Y$, giving us the new position vector of the bead-spring dumbbell at the next timestep.

## A. Solving for Distributions and Material Functions of Rodlike Models

Here we summarise a general numerical method for solving for the transient distribution function of a rodlike model in shear flow based on a spherical harmonic expansion, as originally given by Stewart and Sorensen.[6] The same method can be used for bead-rod dumbbells, multibead-rods[1] and prolate spheroids.[7] In general, we simply require that the distribution function $\psi$ of the system can be characterised by two generalised coordinates (the azimuthal angle $\phi$ and the polar angle $\theta$) and a time constant $\lambda^{(1)}$ which can be derived from the rotational friction of the body (we also have a time constant $\lambda^{(2)}$ which is related to the stress tensor). We can then write the configurational

diffusion equation in shear flow with shear rate $\dot{\gamma}$ as[1,6]

$$\frac{\partial \psi}{\partial t} = \frac{1}{\lambda^{(1)}}\Lambda\psi - \dot{\gamma}\Omega_s\psi \tag{17}$$

where $\Lambda$ and $\Omega_s$ are operators which generalise the diffusion equation given in Eq. (10) for a rodlike model in shear flow. Since $\psi = \psi(\phi, \theta, t)$, we can expand this distribution function as a set of spherical harmonics in the form

$$\psi(\theta, \phi, t) = \frac{1}{4\pi}\sum_{n=0}^{N}\sum_{m=0}^{n}\left[A_{0n}^{m}(t)P_n^m(\cos\theta)\cos(m\phi) + A_{1n}^{m}(t)P_n^m(\cos\theta)\sin(m\phi)\right] \tag{18}$$

where $N$ gives the expansion order, $P_n^m(\cos\theta)$ are the associated Legendre polynomials (such that $P_n^m(\cos\theta)\cos(m\phi)$ or $P_n^m(\cos\theta)\sin(m\phi)$ are spherical harmonics), and the amplitudes $A_{in}^m(t)$ can be solved for via the diffusion equation. The operators $\Lambda$ and $\Omega_s$ both act on spherical harmonics as follows:

$$\Lambda P_n^m s_m = -n(n+1)P_n^m s_m \tag{19a}$$

$$\Lambda P_n^m c_m = -n(n+1)P_n^m c_m \tag{19b}$$

$$\Omega_s P_n^m s_m = \sum_{j=m-2}^{m+2}\sum_{k=n-2}^{n+2} a_{nk}^{mj} P_k^j c_j \; (m > 0) \tag{20a}$$

$$\Omega_s P_n^m c_m = -\sum_{j=m-2}^{m+2}\sum_{k=n-2}^{n+2} a_{nk}^{mj} P_k^j s_j \; (m > 0) \tag{20b}$$

where $s_m \equiv \sin m\phi$, $c \equiv \cos m\phi$, $P_n^m$ is the $n-m$ associated Legendre polynomial acting on $\cos\theta$, and $a_{nk}^{mj}$ are given as follows:

$$a_{n,n-2}^{m,m-2} = \frac{(n-2)(n+m)!\,(1-\delta_{m0})}{4(2n+1)(2n-1)(n+m-4)!} \tag{21a}$$

$$a_{n,n}^{m,m-2} = \frac{3(n-m+2)!(n+m)!\,(1-\delta_{m0})}{4(2n-1)(2n+3)(n+m-2)!(n-m)!} \tag{21b}$$

$$a_{n,n+2}^{m,m-2} = -\frac{(n+3)(n-m+4)!\,(1-\delta_{m0})}{4(2n+1)(2n+3)(n-m)!} \tag{21c}$$

$$a_{n,n}^{m,m} = -m/2 \tag{21d}$$

$$a_{n,n-2}^{m,m+2} = -\frac{(n-2)(1+\delta_{m0})}{4(2n+1)(2n-1)} \tag{21e}$$

$$a_{n,n}^{m,m+2} = -\frac{3(1+\delta_{m0})}{4(2n-1)(2n+3)} \tag{21f}$$

$$a_{n,n+2}^{m,m+2} = \frac{(n+3)(1+\delta_{m0})}{4(2n+1)(2n+3)} \tag{21g}$$

This spherical harmonic expansion along with the above operator defintions creates a set of coupled ODEs, which we have integrated using built-in differential equation solvers in MATLAB.

The unit vector $\boldsymbol{u}$ is given in component form as follows:

$$\boldsymbol{u} = [\cos\phi\sin\theta, \sin\phi\sin\theta, \cos\theta] \tag{22}$$

where $\theta$ is the polar angle and $\phi$ is the azimuthal angle. To calculate material functions for a rodlike model, we use the following form of the stress tensor, written in terms of the unit vector $\boldsymbol{u}$:

$$\boldsymbol{\tau} = -\eta_s\dot{\boldsymbol{\gamma}} - 6nkT\lambda_N^{(2)}\boldsymbol{\kappa} : \langle\boldsymbol{uuuu}\rangle - 3nkT\langle\boldsymbol{uu}\rangle + nkT\boldsymbol{\delta} \tag{23}$$

The averages are given by:

$$\langle\boldsymbol{A}\rangle = \int \boldsymbol{A}\psi d\boldsymbol{u} = \int_0^{\pi}\int_0^{2\pi} \boldsymbol{A}\psi\sin\theta d\phi d\theta \tag{24}$$

and we re-arrange the double dot product $\boldsymbol{\kappa} : \langle\boldsymbol{uuuu}\rangle$ as $\langle(\boldsymbol{\kappa} : \boldsymbol{uu})\boldsymbol{uu}\rangle$. Therefore, for shear stress with $\boldsymbol{\kappa}_{x,y} = \dot{\gamma}$ and all other components 0, we can expanded the stress tensor into averages over sines and cosines as follows:

$$\boldsymbol{\kappa} : \boldsymbol{uuuu} =$$

$$\dot{\gamma}\begin{pmatrix} \cos^3(\phi)\sin(\phi)\sin^4(\theta) & \cos^2(\phi)\sin^2(\phi)\sin^4(\theta) & \cos^2(\phi)\cos(\theta)\sin(\phi)\sin^3(\theta) \\ \cos^2(\phi)\sin^2(\phi)\sin^4(\theta) & \cos(\phi)\sin^3(\phi)\sin^4(\theta) & \cos(\phi)\cos(\theta)\sin^2(\phi)\sin^3(\theta) \\ \cos^2(\phi)\cos(\theta)\sin(\phi)\sin^3(\theta) & \cos(\phi)\cos(\theta)\sin^2(\phi)\sin^3(\theta) & \cos(\phi)\cos^2(\theta)\sin(\phi)\sin^2(\theta) \end{pmatrix} \tag{25}$$

$$\boldsymbol{uu} = \begin{pmatrix} \cos^2(\phi)\sin^2(\theta) & \cos(\phi)\sin(\phi)\sin^2(\theta) & \cos(\phi)\cos(\theta)\sin(\theta) \\ \cos(\phi)\sin(\phi)\sin^2(\theta) & \sin^2(\phi)\sin^2(\theta) & \cos(\theta)\sin(\phi)\sin(\theta) \\ \cos(\phi)\cos(\theta)\sin(\theta) & \cos(\theta)\sin(\phi)\sin(\theta) & \cos^2(\theta) \end{pmatrix} \quad (26)$$

By way of example, if we now specialise to a bead-rod dumbbell with hydrodynamic interaction between the beads given via the RPY tensor (as per Eq. (4) with $Q = L$), we find that:[1]

$$\lambda_2^{(1)}(L,a) = (\zeta L^2/12k_{\mathrm{B}}T)[1-(6a)/(4L)(1+2/3(a/L)^2]^{-1} \quad (27)$$

while

$$\lambda_2^{(2)}(L,a) = (\zeta L^2/12k_{\mathrm{B}}T)[1-(12a)/(4L)(1-2/3(a/L)^2]^{-1} \quad (28)$$

We then further define $\lambda_R^* = (L^2\zeta)/(k_{\mathrm{B}}T)$ (identical to the $\lambda_R^*$ for bead-FF-spring dumbbells, with $L \equiv \sigma$) and $\mu = 1 - 2h_R^*(1-32/27{h_R^*}^2)$ where $h_R^* = (3a)/(4L)$ so that the unit system is indentical to the rodlike non-dimensionalisation of the bead-spring dumbbells. After some algebra, we have for the material functions:

$$\frac{-(\eta-\eta_s)}{nkT\lambda_R^*} = -\frac{6}{5\lambda_R^*\dot{\gamma}}A_{12}^2 - \frac{1}{12\mu}\left[\frac{2}{5}A_{00}^0 - \frac{4}{35}A_{02}^0 + \frac{2}{105}A_{04}^0 - 16A_{04}^4\right] \quad (29a)$$

$$\frac{-\Psi_1}{nkT{\lambda_R^*}^2} = -\frac{12}{5{\lambda_R^*}^2\dot{\gamma}^2}A_{02}^2 - \frac{8}{3\lambda\dot{\gamma}\mu}A_{14}^4 \quad (29b)$$

$$\frac{-\Psi_2}{nkT{\lambda_R^*}^2} = +\frac{3}{{\lambda_R^*}^2\dot{\gamma}^2}\left[-\frac{1}{5}A_{02}^0 - \frac{2}{5}A_{02}^2\right] + \frac{1}{4\lambda\dot{\gamma}\mu}\left[\frac{8}{35}A_{12}^2 - \frac{4}{7}A_{14}^2 - \frac{16}{3}A_{14}^4\right] \quad (29c)$$

$$S = \frac{1}{3}A_{00}^0 - \frac{1}{15}A_{02}^0 + \frac{2}{5}A_{02}^2 \quad (29d)$$

## III. Code Validation

### A. Comparison with FENE Spring Simulations

There is no previous work in the literature on FENE-Fraenkel dumbbells with which we can compare our results, as Larson et al.[8] only report results for 10-bead chains. Therefore, we compare our results with other studies using the semi-implicit predictor-

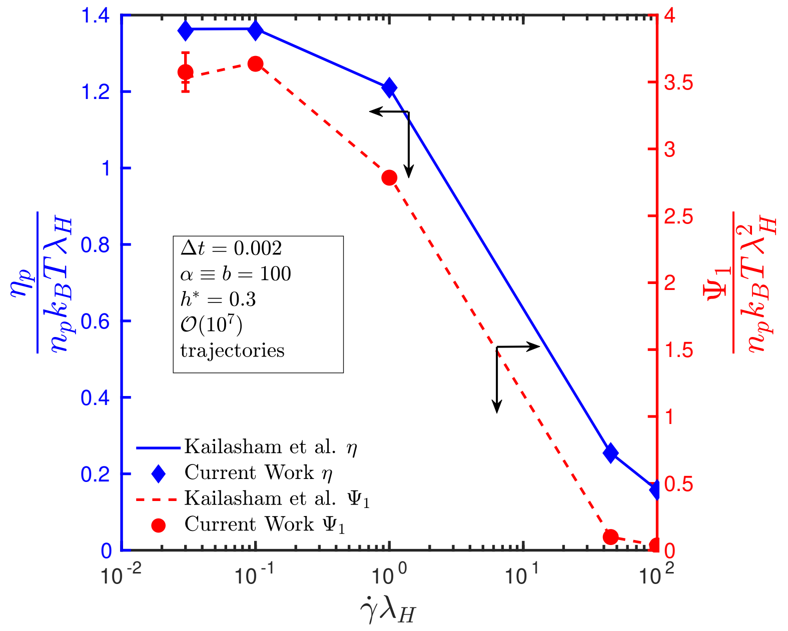


FIG. S2. Comparison of steady-state shear viscosity and first normal stress difference with shear rate against the results of Kailasham et al.[3] Note that with $\sigma = 0$, the $\alpha$ dimensionless parameter used in this paper is equivalent to the dimensionless parameter $b$ characterising the extensibility of a FENE spring. Error bars, when not visible, are smaller than symbol size.

corrector algorithm for FENE dumbbells, as our code should give identical results when setting $\sigma = 0$ in the FENE-Fraenkel force law. One such example is the work by Kailasham et al.,[3] who also used an RPY tensor to mediate hydrodynamic interactions. Some comparisons between their work and our own are shown Fig. S2, with almost perfect agreement.

### B. FENE-Fraenkel Distribution Functions

As an analytical result for the equilibrium end-to-end vector distribution $\psi(\boldsymbol{Q})$ can be derived (section IV), histograms of simulated dumbbell vectors in the absence of flow can be used as an initial check of timestep convergence. The dumbbell vector can be represented in spherical coordinates and the angular distribution plotted separately from the length distribution. An example of the angular distribution is shown in Fig. S3, where the simulated distribution follows the expected sin curve for $\theta$ and is constant for $\phi$. This angular distribution remains spherically symmetric irrespective of the value of $h^*$, $\delta Q$, $H$, $\sigma$ or even the timestep $\Delta t$. This is of course to be expected, as even when

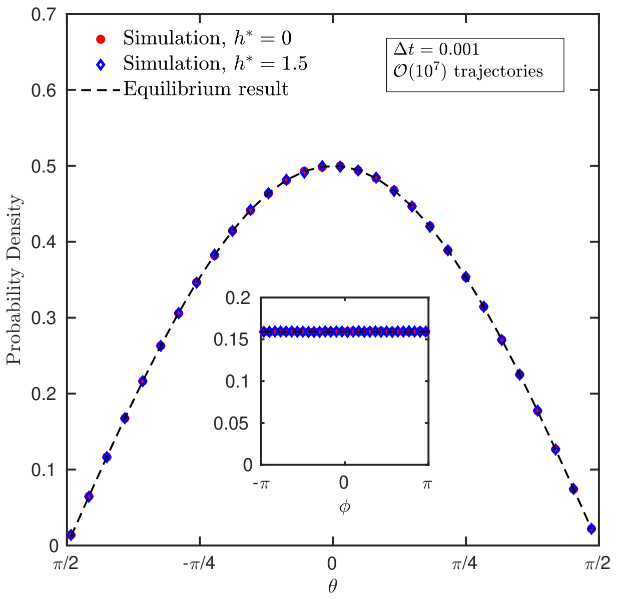


FIG. S3. Comparison of the azimuthal ($\phi$, inset) and polar ($\theta$) angle distributions with those expected at equilibrium, i.e. a perfectly spherical distribution. The simulated distribution is spherical at equilibrium both with and without HI, with error bars smaller than symbol size.

numerically unstable, the algorithm treats all three Cartesian coordinates identically.

The length distribution $\psi(Q)$ is somewhat more complicated, as the distribution function convergence with decreasing $\Delta t$ depends somewhat on the spring parameters $\delta Q$, $H$, $\sigma$, as well as the hydrodynamic interaction parameter $h^*$. In order to analyse the convergence, two measurements are computed. Firstly, the Kolmogorov-Smirnov test, which is a hypothesis test on the null hypothesis that the two distributions are the same. This returns a $p$-value, which we denote $p_{KS}$, such that a large $p_{KS}$ implies that the null hypothesis likely holds, and the two distributions are likely the same. This is simple to calculate in MATLAB using an inbuilt function. Secondly, the summed difference between the analytical and simulated $\psi(Q)$. This is the equivalent of the following integral

$$\mathcal{D}_\psi = \delta Q \int_{-\infty}^{\infty} (\psi_{\text{sim}}(Q) - \psi_{\text{ana}}(Q))^2 dQ = \delta Q \int_{-\infty}^{\infty} (\Delta\psi)^2 dQ \tag{30}$$

which in discrete form, with the simulated lengths binned into $N_{\text{bin}}$ segments, is

$$\mathcal{D}_\psi = \delta Q \sum_{i}^{N_{\text{bins}}} (\psi_{\text{sim}}(Q_i) - \psi_{\text{ana}}(Q_i))^2 (\Delta Q_i) = \delta Q \sum_{i}^{N_{\text{bins}}} (\Delta\psi_i)^2 (\Delta Q_i) \tag{31}$$

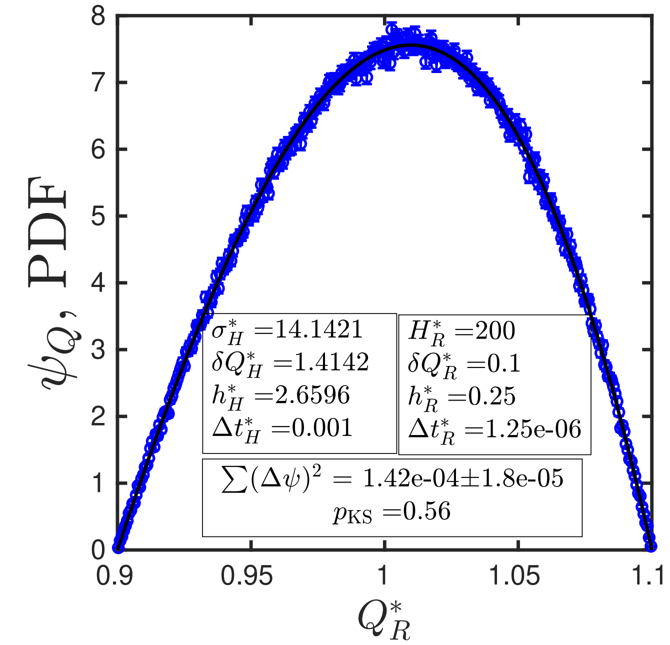


(a)

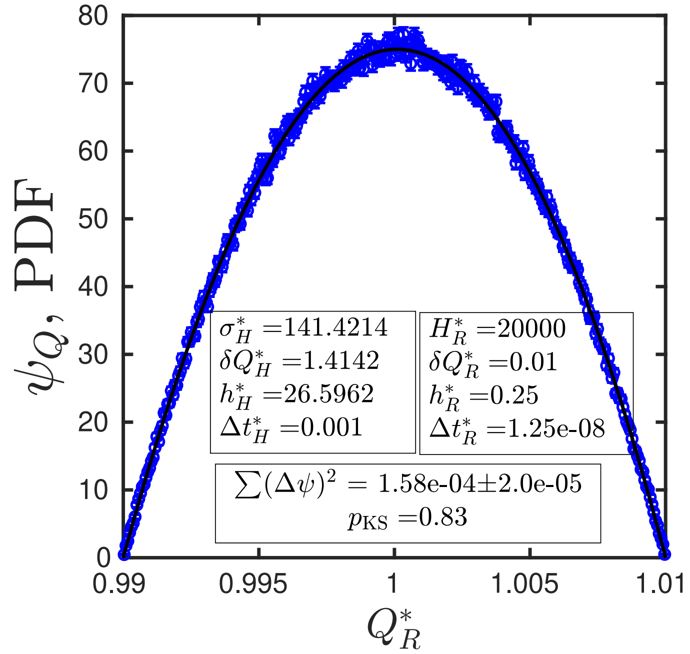


(b)

FIG. S4. Distribution functions at two values of $\delta Q^*_R$.

where $\mathcal{D}_\psi$ is the 'summed difference', denoted $\sum(\Delta\psi)^2$ in Fig. S4. Note the multiplication by $\delta Q$, which is necessary to non-dimensionalise the summed difference. Since $\Delta\psi$ has units of inverse length, a direct integral over this quantity squared will have units of inverse length, so it must be multiplied by a quantity with units of length to

obtain a dimensionless form. By multiplying by $\delta Q$, the summed difference should be independent of the specific choice of $\delta Q$, but instead simply a function of the difference in shape between the two distributions. For example, see Fig. S4, which shows two plots with the same $\Delta t^*_H$, $\delta Q^*_H$ and $h^*_R$. Both plots are converged by the Kolmogorov-Smirnov test, but if they were not normalised by $\delta Q^*_R$, the calculated differences would differ by an order of magnitude. Essentially, this ensures that with identical binning and sample size, two distributions which are similarly 'accurate' should give similar summed differences, irrespective of the FENE-Fraenkel spring parameters.

The error in this summed difference can also be computed, by assuming the counts in each bin are Poisson-distributed, and hence the error in each measurement is the square root of the bin count, normalised by the same factor $c$ as to transform from raw counts to a PDF.

$$\sigma_{\text{bin}} = \sqrt{n}/c \tag{32}$$

The total error is then, when propagated:

$$\sigma_T = \sqrt{\sum_i^{N_{\text{bins}}} (2\Delta\psi_i \Delta Q_i \sigma_{\text{bin},i})^2} \tag{33}$$

## IV. Analytical Results

We begin with the spring potential of the dumbbell, which is:

$$\phi_{\text{eq}} = -\frac{H\delta Q^2}{2} \ln\left[1 - \frac{(Q-\sigma)^2}{\delta Q^2}\right] \tag{34}$$

In general, the distribution function has the form (in spherical coordinates):[1]

$$\psi_{\text{eq}}(Q) = \frac{Q^2 e^{-\phi_{\text{eq}}/k_{\text{B}}T}}{4\pi J_{\text{eq}}} \tag{35}$$

where $J_{\text{eq}}$ is a normalisation factor (after already integrating over the isotropic angular distribution, giving the $4\pi$ factor). The normalisation must be over all possible values of Q, which in this case has one upper bound, $\sigma + \delta Q$ and two possible lower bounds, the larger of 0 and $\sigma - \delta Q$. For now we will restrict our calculation to the $\sigma - \delta Q$ lower

bound. The normalisation factor will have the form:

$$J_{\text{eq}} = \int_{\sigma-\delta Q}^{\sigma+\delta Q} \left[1 - \frac{(Q-\sigma)^2}{\delta Q^2}\right]^{\frac{H\delta Q^2}{2k_{\text{B}}T}} Q^2 dQ \tag{36}$$

We can split this integral into two halves as follows:

$$A_1 = \int_{\sigma}^{\sigma+\delta Q} \left[1 - \frac{(Q-\sigma)^2}{\delta Q^2}\right]^{c} Q^2 dQ \tag{37a}$$

$$A_2 = \int_{\sigma-\delta Q}^{\sigma} \left[1 - \frac{(Q-\sigma)^2}{\delta Q^2}\right]^{c} Q^2 dQ \tag{37b}$$

$$J_{\text{eq}} = A_1 + A_2 \tag{37c}$$

where we have set $c = H\delta Q^2/2k_{\text{B}}T$. For $A_1$, we make the substitution $t = (Q-\sigma)^2/\delta Q^2$, so that $Q = \sigma + \delta Q\sqrt{t}$, $dQ = 2\sqrt{t}/\delta Q dt$, and the integral becomes:

$$A_1 = \int_0^1 (1-t)^c (\delta Q\sqrt{t} + \sigma)^2 \frac{\delta Q}{2\sqrt{t}} dt \tag{38}$$

For $A_2$, we can make the same substitution $t = (Q - \sigma + \delta Q)^2/\delta Q^2$, only we use the other solution for $Q$, giving $Q = \sigma - \delta Q\sqrt{t}$, $dQ = -2\sqrt{t}/\delta Q dt$, so that the integral is:

$$A_2 = \int_1^0 (1-t)^c (-\delta Q\sqrt{t} + \sigma)^2 \frac{-\delta Q}{2\sqrt{t}} dt \tag{39}$$

While it is possible to expand the brackets and manipulate the integrals into a form which is equivalent to the Beta function, Mathematica can symbolically solve the combined integral for us, giving:

$$J_{\text{eq}} = \frac{\delta Q(\delta Q^2 + (3+2c)\sigma^2)}{3+2c} \text{B}\left(\frac{1}{2}, 1+c\right) \tag{40}$$

With this Mathematica script, it is trivial to compute equilibrium averages over $Q$, such as:

$$\langle Q^2 \rangle_{\text{eq}} = \frac{\delta Q(3\delta Q^4 + 6(5-2c)\delta Q^2\sigma^2 + (-5+2c)(-3+2c)\sigma^4)}{(5-2c)(3-2c)} \text{B}\left(\frac{1}{2}, 1-c\right) \tag{41}$$

## V. Selection of Parameters for Experimental Comparisons

### A. Choosing Bead Radius

Here we show how bead radii are calculated for the FENE-Fraenkel spring to properly compare with experimental results for rigid macromolecules as in section 3.4 of the main paper. This is performed primarily based on the results in section 14.6 of Dynamics of Polymeric Liquids Vol.2 by Bird et al.[1] The full form of Eq. (17) for a multibead-rod is given in Bird et al. by Eq. (14.6-13), which is as follows:

$$\frac{\partial}{\partial t}\psi = \frac{1}{6\lambda_N^{(1)}}\left(\frac{\partial}{\partial \boldsymbol{u}}\cdot\frac{\partial}{\partial \boldsymbol{u}}\psi\right) - \left(\frac{\partial}{\partial \boldsymbol{u}}\cdot[\boldsymbol{\kappa}\cdot\boldsymbol{u} - \boldsymbol{\kappa}:\boldsymbol{uuu}]\psi\right) \tag{42}$$

with the stress tensor given by:

$$\boldsymbol{\tau} = -\eta_s\dot{\boldsymbol{\gamma}} - 6nkT\lambda_N^{(2)}\boldsymbol{\kappa}:\langle\boldsymbol{uuuu}\rangle - 3nkT\langle\boldsymbol{uu}\rangle + nkT\boldsymbol{\delta} \tag{43}$$

with $\lambda_N^{(2)}$ and $\lambda_N^{(1)}$ defined as:

$$\lambda_N^{(1)}(h_N^*,\xi) = \frac{\zeta d^2}{12kT}\left(\sum_{v=-(N-1)}^{N-1} v\phi_v\left(h_N^*,\xi^2,N\right)\right) \tag{44}$$

$$\lambda_N^{(2)}(h_N^*,\xi) = \frac{\zeta d^2}{12kT}\left(\sum_{v=-(N-1)}^{N-1} v\phi_v\left(2h_N^*,-\xi^2,N\right)\right) \tag{45}$$

with $\phi_v$ defined by the following equation:

$$\phi_v(\alpha,\beta,N) + 2\alpha\sum_{\mu}{}' \left(\frac{1}{|v-\mu|} +_3^2 \beta_{|v-\mu|^3}\right)\phi_\mu(\alpha,\beta,N) = \frac{1}{2}v \tag{46}$$

where $\sum_\mu'$ runs over $-(N-1)$ to $+(N+1)$, omitting terms $\mu=\nu$ and using even (odd) values of $\mu$ if N is odd (even). The parameters are $\xi = a/d$ where $a$ is the bead radius and $d$ is the distance between bead centers, $N$ is the number of beads, $L = d(N-1)$ is the total length of the rod, and $h_N^*$ is given as $h_N^* = \zeta/8\pi\eta_s d$.

These expressions can be solved for the values of $\lambda_N^{(1)}$, which essentially defines

the rotational friction of the molecule, and $\lambda_N^{(2)}$, which gives the stress response to orientation. Note that explicit expressions have already been given in Eqs. (27) and (28) for a bead-rod dumbbell (the $N = 2$ case), albeit with slightly different definitions of $L$ and $h_N^*$. The key is that for purely orientational measurements, such as the $S$-parameter characterising Linear Dichroism, the effective bead radius for the bead-rod dumbbell can be chosen such that $\lambda_2^{(1)} = \lambda_N^{(1)}$, meaning that the diffusion equation for the two cases is identical. This same bead radius can then be used for FENE-Fraenkel simulations to give a spring which approximately behaves hydrodynamically like a multibead-rod.

For viscosity measurements, the situation is slightly more complicated. In this case, it's not possible to choose a single bead radius such that both $\lambda_2^{(1)} = \lambda_N^{(1)}$ and $\lambda_2^{(2)} = \lambda_N^{(2)}$. Therefore, the bead radius was chosen to sit somewhere between the radius such that $\lambda_2^{(1)} = \lambda_N^{(1)}$ and the radius such that $\lambda_2^{(2)} = \lambda_N^{(2)}$, so that the bead-rod viscosity data gives a reasonable fit to the multibead-rod viscosity data. This is able to once again give a reasonable overall hydrodynamic approximation of a multibead-rod, as can be seen in Fig. (18) of the main paper.

## References


[1] R. B. Bird, C. F. Curtiss, R. C. Armstrong, and O. Hassager, *Dynamics of Polymeric Liquids - Volume 2: Kinetic Theory*, 2nd ed. (John Wiley, New York, 1987).

[2] H. C. Öttinger, *Stochastic processes in polymeric fluids: Tools and examples for developing simulation algorithms* (Springer-Verlag, Berlin Heidelberg, 1996).

[3] R. Kailasham, R. Chakrabarti, and J. R. Prakash, "Rheological consequences of wet and dry friction in a dumbbell model with hydrodynamic interactions and internal viscosity," J. Chem. Phys. **149**, 094903 (2018).

[4] C. C. Hsieh, L. Li, and R. G. Larson, "Modeling hydrodynamic interaction in brownian dynamics: Simulations of extensional flows of dilute solutions of DNA and polystyrene," J. Non-Newtonian Fluid Mech. **113**, 147–191 (2003).

[5] R. Prabhakar and J. R. Prakash, "Multiplicative separation of the influences of excluded volume, hydrodynamic interactions and finite extensibility on the rheological

properties of dilute polymer solutions," J. Non-Newtonian Fluid Mech. **116**, 163–182 (2004).

[6]W. E. Stewart and J. P. Sorensen, "Hydrodynamic interaction effects in rigid dumbbell suspensions. II. Computations for steady shear flow," Trans. Soc. Rheol. **16**, 1–13 (1972).

[7]J. R. McLachlan, D. J. Smith, N. P. Chmel, and A. Rodger, "Calculations of flow-induced orientation distributions for analysis of linear dichroism spectroscopy," Soft Matter **9**, 4977–4984 (2013).

[8]C. C. Hsieh, S. Jain, and R. G. Larson, "Brownian dynamics simulations with stiff finitely extensible nonlinear elastic-Fraenkel springs as approximations to rods in bead-rod models," J. Chem. Phys. **124** (2006).
